# Supplementary material for: Flame: Simplifying Topology Extension in Federated Learning
Source: arXiv:2305.05118 source file (2024-01-17)
Supplement: Supplementary file 1 [file appendix.tex]

\section{Appendix}

\begin{table*}[t!]
  \small
  \ra{1.2}
  \begin{tabular}{c  c  c  c  c  c}
    \toprule
    \multicolumn{2}{c}{\textbf{Feature}} & \textbf{\sys (ours)} & \textbf{FedML~\cite{fedml}} & \textbf{Flower~\cite{flower}} & \textbf{FedScale~\cite{fedscale}}
    \\
    \midrule
    \multirow{7}{*}{Topology} & Classical FL~\cite{fedavg} & \cmark & \cmark & \cmark & \cmark
    \\
    & Hierarchical FL~\cite{hierFAVG_topology} & \cmark & \cmark & \xmark & \xmark
    \\
    & Distributed FL~\cite{fedml} & \cmark & \cmark & \xmark & \xmark
    \\
    & Hybrid FL~\cite{hybrid_fl} & \cmark & \xmark & \xmark & \xmark
    \\
    & Coordinated FL~\cite{fl_at_scale} & \cmark$^*$ & \xmark & \xmark & \xmark
    \\
    & Vertical FL~\cite{vfl} & \xmark & \cmark & \xmark & \xmark
    \\
    & Async Hierarchical FL & \cmark & \xmark & \xmark & \xmark
    \\
    & Async Coordinated FL & \cmark & \xmark & \xmark & \xmark
    \\
    \midrule
    \multirow{4}{*}{Protocol} & gRPC & \cmark & \cmark & \cmark & \cmark
    \\
    & MQTT & \cmark & \cmark & \xmark & \xmark
    \\
    & MPI & \xmark & \cmark & \xmark & \xmark 
    \\
    & NCCL & \xmark & \cmark & \xmark & \xmark 
    \\
    \midrule
    \multirow{2}{*}{Aggregation Policy} & Synchronous FL~\cite{fedavg} & \cmark & \cmark & \cmark & \cmark
    \\
    & Asynchronous FL~\cite{fedbuff} & \cmark & \cmark$^\dag$ & \xmark & \cmark
    \\
    \midrule
	\multirow{10}{*}{Algorithm$^\ddag$} & FedAvg~\cite{fedavg} & \cmark & \cmark & \cmark & \cmark
    \\
    & FedProx~\cite{fedprox} & \cmark & \cmark & \cmark & \cmark
    \\
    & FedAdam~\cite{fedopt} & \cmark & \xmark & \cmark & \xmark
    \\
    & FedAdagrad~\cite{fedopt} & \cmark & \xmark & \cmark & \xmark
    \\
    & FedYogi~\cite{fedopt} & \cmark & \xmark & \cmark & \cmark
    \\
    & FedDyn~\cite{feddyn} & \cmark & \cmark & \xmark & \xmark
    \\
    & FedBuff$^\S$~\cite{fedbuff} & \cmark & \cmark$^\dag$ & \xmark & \cmark
    \\
    & SCAFFOLD~\cite{scaffold} & \xmark & \cmark & \xmark & \xmark
    \\
    & q-FedAvg~\cite{qfedavg} & \xmark & \xmark & \cmark & \cmark
    \\
    & FedNova~\cite{fednova} & \xmark & \cmark & \cmark & \xmark
    \\
    \midrule
    \multirow{4}{*}{Client Selection} & Select All & \cmark & \cmark & \cmark & \cmark
    \\
    & Random~\cite{fedavg} & \cmark & \cmark & \cmark & \cmark
    \\
    & FedBuff$^\S$~\cite{fedbuff} & \cmark & \cmark$^\dag$ & \xmark & \cmark
    \\
    & Oort~\cite{oort_selection} & \cmark & \xmark & \xmark & \cmark
    \\
    \midrule
    \multirow{2}{*}{Sample Selection} & Select All & \cmark & \cmark & \cmark & \cmark
    \\
    & FedBalancer~\cite{fedbalancer} & \cmark & \xmark & \xmark & \xmark
    \\
    \midrule
    \multirow{2}{*}{Security} & Differential Privacy~\cite{dp} & \cmark & \cmark & \cmark & \cmark
    \\
    & Secure Aggregation~\cite{secureagg} & \xmark & \cmark & \xmark & \xmark
    \\
    \bottomrule
  \end{tabular}
  \caption{Comparing \sys with other FL frameworks. $^\dag$: simulation;
    $^*$: simplified version of an original architecture; $^\ddag$: widely
    used algorithms listed; others (e.g., FedML) implemented several
    other algorithms (omitted for brevity); $^\S$: both aggregation
    algorithm and client selection are included.}
  \label{tbl:flframework_comparison}
\end{table*}

\tref{tbl:flframework_comparison} provides a summary of the key features of existing FL frameworks, based on their public repositories as of May 5th, 2023. While the table showcases \sys's strengths in comparison to other frameworks, it is not intended to be exhaustive. For instance, FedML offers several other algorithms and FedScale offers other features such as cohort-based learning~\cite{auxo}. Although we took great care in conducting code analysis, we encountered ambiguities in certain aspects during the comparison. We encourage the readers to explore the complete list of features offered by each framework through their project web page or GitHub repositories.
